# Supplementary material for: Nematic spin liquid in a spin-1 pyrochlore magnet and its realization in $\mathrm{NaCaNi}_2\mathrm{F}_7$
Source: arXiv:2503.12776 source file (2026-02-27)
Supplement: Supplementary file 1 [file supplemental.pdf]

*Supplemental Material for*  
**Abundance of spin liquids in the  $S = 1$  bilinear-biquadratic model**  
**on the pyrochlore lattice, and its application to  $\text{NaCaNi}_2\text{F}_7$**

Rico Pohle<sup>1</sup> and Nic Shannon<sup>2</sup>

<sup>1</sup>*Institute for Materials Research, Tohoku University, Sendai, Miyagi 980-8577, Japan*

<sup>2</sup>*Theory of Quantum Matter Unit, Okinawa Institute of Science and Technology Graduate University, Onna-son, Okinawa 904-0412, Japan*  
(Dated: March 16, 2025)

## I. DETAILS OF THE $U(3)$ METHOD

Spin-1 moments contain both magnetic dipole and quadrupole components on a single site. To fully capture all spin degrees of freedom associated with an  $S = 1$  moment, we adopt the  $U(3)$  formalism, as described in detail in Ref. [1]. Ground state properties are determined through variational energy minimization using the machine learning library JAX [2], while finite-temperature properties are computed via semiclassical Monte Carlo simulations (u3MC). Dynamical properties were obtained through molecular dynamics simulations (u3MD) by numerically integrating the corresponding equations of motion. In the following Sections, we provide a brief overview of the mathematical background and the numerical implementation of each of these methods.

### A. Spin-1 magnets within the $U(3)$ formalism

We express the quantum state of the spin-1 moments on a given lattice site in terms of the  $3 \times 3$  Hermitian matrix

$$\mathcal{A}_\beta^\alpha = (\mathbf{d}^\alpha)^* \mathbf{d}_\beta, \quad (\text{S1})$$

which we call henceforth  $\mathcal{A}$  matrix. The  $\mathcal{A}$  matrices can be written in terms of complex vectors  $\mathbf{d}$

$$\mathbf{d} = \begin{pmatrix} x_1 + i x_2 \\ x_3 + i x_4 \\ x_5 + i x_6 \end{pmatrix}, \quad (\text{S2})$$

which are sometimes referred to as directors [1, 3, 4]. We implicitly enforce the unit norm constraint on the directors

$$\mathbf{d}^* \mathbf{d} = |\mathbf{d}|^2 = 1, \quad (\text{S3})$$

by parametrizing their components equidistantly on a five-dimensional sphere

$$\begin{aligned} x_1 &= \theta_2^{1/4} \theta_1^{1/2} \sin \phi_1, \\ x_2 &= \theta_2^{1/4} \theta_1^{1/2} \cos \phi_1, \\ x_3 &= \theta_2^{1/4} (1 - \theta_1)^{1/2} \sin \phi_2, \\ x_4 &= \theta_2^{1/4} (1 - \theta_1)^{1/2} \cos \phi_2, \\ x_5 &= (1 - \theta_2^{1/2})^{1/2} \sin \phi_3, \\ x_6 &= (1 - \theta_2^{1/2})^{1/2} \cos \phi_3, \end{aligned} \quad (\text{S4})$$

with  $0 \leq \theta_1, \theta_2 \leq 1$  and  $0 \leq \phi_1, \phi_2, \phi_3 < 2\pi$ . The unphysical gauge can be fixed by setting the  $z$  component of  $\mathbf{d}$  to purely real values, i.e.,  $\phi_3 = \pi/2$ , which leaves a total of four degrees of freedom, as expected for a spin-1 moment [1, 5].

The information about dipole and quadrupole components are simultaneously incorporated in the  $\mathcal{A}$  matrix and can be extracted using the following expressions:

$$S_i^\alpha = -i \epsilon_{\beta}^{\alpha \gamma} \mathcal{A}_{i\gamma}^\beta, \quad (\text{S5})$$

$$Q_{i\beta}^\alpha = -\mathcal{A}_{i\beta}^\alpha - \mathcal{A}_{i\alpha}^\beta + \frac{2}{3} \delta^{\alpha\beta} \mathcal{A}_{i\gamma}^\gamma, \quad (\text{S6})$$

where  $\epsilon_{\beta}^{\alpha \gamma}$  is the Levi-Civita symbol, and  $\delta^{\alpha\beta}$  is the Kronecker delta. We adopt the Einstein convention of summing over repeated indices, and express spin quadrupoles in their symmetric and traceless rank-2 tensor form.

Using Eqs. (S5) and (S6) we rewrite the bilinear biquadratic (BBQ) model,  $\mathcal{H}_{\text{BBQ}}$ , in Eq. (1) of the main text in its purely bilinear form

$$\mathcal{H}_{\text{BBQ}} = \sum_{\langle ij \rangle} \left[ J \mathcal{A}_{i\beta}^\alpha \mathcal{A}_{j\alpha}^\beta + (K - J) \mathcal{A}_{i\beta}^\alpha \mathcal{A}_{j\beta}^\alpha + K \mathcal{A}_{i\alpha}^\alpha \mathcal{A}_{j\beta}^\beta \right]. \quad (\text{S7})$$

For convenience, the dipole and quadrupole components can be directly obtained from the  $\mathcal{A}$  matrices using the following relation:

$$\begin{pmatrix} \mathbf{S}^2 \\ S^x \\ S^y \\ S^z \\ Q^{x^2-y^2} \\ Q^{3z^2-r^2} \\ Q^{xy} \\ Q^{xz} \\ Q^{yz} \end{pmatrix} = C \begin{pmatrix} \mathcal{A}_1^1 \\ \mathcal{A}_2^1 \\ \mathcal{A}_3^1 \\ \mathcal{A}_2^2 \\ \mathcal{A}_2^3 \\ \mathcal{A}_3^2 \\ \mathcal{A}_3^3 \end{pmatrix}, \quad (\text{S8})$$

where the spin-length constraint is  $\mathbf{S}^2 = S(S+1) = 2$ , and  $C$  is the  $9 \times 9$  transformation matrix given by:

$$C = \begin{pmatrix} 2 & 0 & 0 & 0 & 2 & 0 & 0 & 0 & 2 \\ 0 & 0 & 0 & 0 & 0 & -i & 0 & i & 0 \\ 0 & 0 & i & 0 & 0 & 0 & -i & 0 & 0 \\ 0 & -i & 0 & i & 0 & 0 & 0 & 0 & 0 \\ -1 & 0 & 0 & 0 & 1 & 0 & 0 & 0 & 0 \\ \frac{1}{\sqrt{3}} & 0 & 0 & 0 & \frac{1}{\sqrt{3}} & 0 & 0 & 0 & -\frac{2}{\sqrt{3}} \\ 0 & -1 & 0 & -1 & 0 & 0 & 0 & 0 & 0 \\ 0 & 0 & -1 & 0 & 0 & 0 & -1 & 0 & 0 \\ 0 & 0 & 0 & 0 & 0 & -1 & 0 & -1 & 0 \end{pmatrix}. \quad (\text{S9})$$

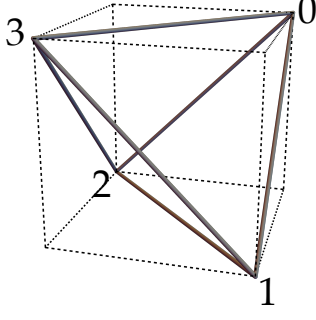

Figure S1. Site indices for a single tetrahedron in the pyrochlore lattice, consistent with Eq. (S17).

The components of the dipole vector are expressed as:

$$\mathbf{S}_i = \begin{pmatrix} S_i^x \\ S_i^y \\ S_i^z \end{pmatrix}, \quad (\text{S10})$$

and the components of the quadrupole vector are expressed as:

$$\mathbf{Q}_i = \begin{pmatrix} Q_i^{x^2-y^2} \\ Q_i^{3z^2-r^2} \\ Q_i^{xy} \\ Q_i^{xz} \\ Q_i^{yz} \end{pmatrix} = \begin{pmatrix} \frac{1}{2} (Q_{ix}^x - Q_{iy}^y) \\ \frac{1}{\sqrt{3}} (Q_{iz}^z - \frac{1}{2} (Q_{ix}^x + Q_{iy}^y)) \\ Q_{iy}^x \\ Q_{iz}^x \\ Q_{iz}^y \end{pmatrix}. \quad (\text{S11})$$

By using the commutation relations for  $\mathcal{A}$  matrices

$$\begin{aligned} [\mathcal{A}_{i\beta}^\alpha, \mathcal{A}_{i\eta}^\gamma] &= \delta_{\beta\eta}^\gamma \mathcal{A}_{i\eta}^\alpha - \delta_{\eta\beta}^\alpha \mathcal{A}_{i\beta}^\gamma, \\ [\mathcal{A}_{i\beta}^\alpha, \mathcal{A}_{j\eta}^\gamma] &= 0, \end{aligned} \quad (\text{S12})$$

we obtain the equations of motion for the BBQ model, Eq. (S7)

$$\begin{aligned} \frac{d}{dt} \mathcal{A}_{i\eta}^\gamma &= -i [\mathcal{A}_{i\eta}^\gamma, \mathcal{H}_{\text{BBQ}}] \\ &= -i \sum_{\delta} \left[ J \left( \mathcal{A}_{i\alpha}^\gamma \mathcal{A}_{i+\delta,\eta}^\alpha - \mathcal{A}_{i\eta}^\alpha \mathcal{A}_{i+\delta,\alpha}^\gamma \right) \right. \\ &\quad \left. + (K - J) \left( \mathcal{A}_{i\alpha}^\gamma \mathcal{A}_{i+\delta,\alpha}^\eta - \mathcal{A}_{i\eta}^\alpha \mathcal{A}_{i+\delta,\gamma}^\alpha \right) \right], \end{aligned} \quad (\text{S13})$$

where  $\sum_{\delta}$  sums over the nearest neighbors of site  $i$ . The results for dynamics shown in Fig. 4 of the main text were obtained by numerically integrating Eq. (S13), using the methods described in Section IF.

## B. Anisotropic interactions for $\text{NaCaNi}_2\text{F}_7$

To simulate dynamical properties for  $\text{NaCaNi}_2\text{F}_7$ , we generalize  $\mathcal{H}_{\text{BBQ}}$ , in Eq. (S7) to

$$\begin{aligned} \mathcal{H}_{\text{NaCaNi}_2\text{F}_7} &= \sum_{\langle ij \rangle} \left( J_{\beta\nu}^{\alpha\mu} \right)_{ij} \mathcal{A}_{i\beta}^\alpha \mathcal{A}_{j\nu}^\mu \\ &\quad + J_{2\text{nd}} \sum_{\langle\langle i,j \rangle\rangle} \mathcal{A}_{i\beta}^\alpha (\mathcal{A}_{j\alpha}^\beta - \mathcal{A}_{j\beta}^\alpha), \end{aligned} \quad (\text{S14})$$

to describe a bond-dependent spin-anisotropic interaction tensor,  $\left( J_{\beta\nu}^{\alpha\mu} \right)_{ij}$ , on nearest-neighboring sites, and isotropic second nearest-neighbor interactions  $J_{2\text{nd}}$ . We construct the interaction tensor,  $\left( J_{\beta\nu}^{\alpha\mu} \right)_{ij}$ , after the transformation using Eq. (S9)

$$\left( J_{\beta\nu}^{\alpha\mu} \right)_{ij} = C^{-1} \left( \tilde{J}_{\beta\nu}^{\alpha\mu} \right)_{ij} C, \quad (\text{S15})$$

where  $\tilde{J}_{\beta\nu}^{\alpha\mu}$  contains spin-dipole and spin-quadrupole interactions in the following form:

$$\left( \tilde{J}_{\beta\nu}^{\alpha\mu} \right)_{ij} = \begin{pmatrix} [0]_{1 \times 1} & \mathbf{0} & \mathbf{0} \\ \mathbf{0} & [\tilde{J}_{ij}^S]_{3 \times 3} & \mathbf{0} \\ \mathbf{0} & \mathbf{0} & [\tilde{J}_{ij}^Q]_{5 \times 5} \end{pmatrix}. \quad (\text{S16})$$

In this work, we consider anisotropies only between spin-dipoles

$$\begin{aligned} \hat{J}_{01}^S &= \begin{pmatrix} J_2 & J_4 & J_4 \\ -J_4 & J_1 & J_3 \\ -J_4 & J_3 & J_1 \end{pmatrix}, \quad \hat{J}_{23}^S = \begin{pmatrix} J_2 & -J_4 & J_4 \\ J_4 & J_1 & -J_3 \\ -J_4 & -J_3 & J_1 \end{pmatrix}, \\ \hat{J}_{02}^S &= \begin{pmatrix} J_1 & -J_4 & J_3 \\ J_4 & J_2 & J_4 \\ J_3 & -J_4 & J_1 \end{pmatrix}, \quad \hat{J}_{13}^S = \begin{pmatrix} J_1 & J_4 & -J_3 \\ -J_4 & J_2 & J_4 \\ -J_3 & -J_4 & J_1 \end{pmatrix}, \\ \hat{J}_{03}^S &= \begin{pmatrix} J_1 & J_3 & -J_4 \\ J_3 & J_1 & -J_4 \\ J_4 & J_4 & J_2 \end{pmatrix}, \quad \hat{J}_{12}^S = \begin{pmatrix} J_1 & -J_3 & J_4 \\ -J_3 & J_1 & -J_4 \\ -J_4 & J_4 & J_2 \end{pmatrix}, \end{aligned} \quad (\text{S17})$$

defined on the bonds connecting sites  $i$  and  $j$  (see Fig. S1), following the same convention used in Yan *et al.* [6]. Interactions between spin-quadrupoles are treated isotropic where

$$\hat{J}_{ij}^Q = K \cdot \mathbf{1}_{5 \times 5}, \quad (\text{S18})$$

for all nearest-neighbor bonds  $ij$ .

In this form we extend the equations of motion in Eq. (S13) to

$$\begin{aligned}
\frac{d}{dt} \mathcal{A}_{i\eta}^\gamma &= -i [\mathcal{A}_{i\eta}^\gamma, \mathcal{H}_{\text{NaCaNi}_2\text{F}_7}] \\
&= -i \sum_{\delta \in \text{nn}} \left[ \left( J_{\beta\nu}^{\eta\mu} \right)_{i,i+\delta} \mathcal{A}_{i\beta}^\gamma - \left( J_{\gamma\nu}^{\alpha\mu} \right)_{i,i+\delta} \mathcal{A}_{i\eta}^\alpha \right] \mathcal{A}_{i+\delta,\nu}^\mu \\
&\quad - i J_{2\text{nd}} \sum_{\delta' \in \text{nnn}} \left[ \mathcal{A}_{i\beta}^\gamma \left( \mathcal{A}_{i+\delta',\eta}^\beta - \mathcal{A}_{i+\delta',\beta}^\eta \right) + \mathcal{A}_{i\eta}^\beta \left( \mathcal{A}_{i+\delta',\gamma}^\beta - \mathcal{A}_{i+\delta',\beta}^\gamma \right) \right].
\end{aligned} \tag{S19}$$

The results for dynamics shown in Fig. 5 of the main text, and Fig. S6, Fig. S7 below, were obtained by numerically integrating Eq. (S19), using the methods described in Section IF.

### C. Characterisation of Spin liquids

#### 1. Bond correlation functions

The BBQ model defined in Eq. (S7) exhibits a total of seven spin liquid phases, five of which also occur in the ground state, as summarized in Fig. 1 of the main text. Spin liquids are typically challenging to observe and distinguish using conventional magnetic order parameters or thermodynamic quantities such as the specific heat alone. Thus, to better characterize these phases, we introduce bond correlation functions, following Refs. [7–10], which distinguish spin liquids based on the irreducible representations (irreps) associated with their local correlations (constraint).

We consider the primitive four-site unit cell of the pyrochlore lattice (see Fig. S1) and define bond variables,  $\rho_{ij}$ , which are equivalent to  $\mathbf{S}_i \cdot \mathbf{S}_j$  for spin dipoles, and  $\mathbf{Q}_i \cdot \mathbf{Q}_j$  for spin quadrupoles. These bond variables transform according to the irreps  $A_1$ ,  $E$ , and  $T_2$  under the symmetry group  $\mathcal{T}_d$

$$\begin{pmatrix} \Lambda_{A_1} \\ \Lambda_{E,1} \\ \Lambda_{E,2} \\ \Lambda_{T_2,1} \\ \Lambda_{T_2,2} \\ \Lambda_{T_2,3} \end{pmatrix}^\rho = \begin{pmatrix} \frac{1}{\sqrt{6}} & \frac{1}{\sqrt{6}} & \frac{1}{\sqrt{6}} & \frac{1}{\sqrt{6}} & \frac{1}{\sqrt{6}} & \frac{1}{\sqrt{6}} \\ \frac{1}{\sqrt{3}} & \frac{1}{2\sqrt{3}} & \frac{1}{2\sqrt{3}} & \frac{1}{2\sqrt{3}} & \frac{1}{2\sqrt{3}} & \frac{1}{\sqrt{3}} \\ 0 & \frac{1}{2} & -\frac{1}{2} & -\frac{1}{2} & \frac{1}{2} & 0 \\ 0 & 0 & \frac{1}{\sqrt{2}} & \frac{1}{\sqrt{2}} & 0 & 0 \\ 0 & \frac{1}{\sqrt{2}} & 0 & 0 & \frac{1}{\sqrt{2}} & 0 \\ \frac{1}{\sqrt{2}} & 0 & 0 & 0 & 0 & \frac{1}{\sqrt{2}} \end{pmatrix} \begin{pmatrix} \rho_{0,1} \\ \rho_{0,2} \\ \rho_{0,3} \\ \rho_{1,2} \\ \rho_{1,3} \\ \rho_{2,3} \end{pmatrix}. \tag{S20}$$

Then, the bond correlator

$$\lambda_\nu^\rho = \frac{4}{N} \sum_{\triangle} (\Lambda_\nu^\rho)^2, \tag{S21}$$

identifies dominant correlations in dipole and quadrupole channels,  $\rho = \{S, Q\}$ , of irrep  $\nu = \{A_1, E, T_2\}$ . For multidimensional irreps, we use the vector representations  $\Lambda_E = (\Lambda_{E,1}, \Lambda_{E,2})$  and  $\Lambda_{T_2} = (\Lambda_{T_2,1}, \Lambda_{T_2,2}, \Lambda_{T_2,3})$ . The associated susceptibility of the bond correlator in Eq. (S21) is then given by

$$\chi[\lambda_\nu^\rho] = \frac{N}{T} \left[ \langle (\lambda_\nu^\rho)^2 \rangle - \langle \lambda_\nu^\rho \rangle^2 \right]. \tag{S22}$$

where  $\langle \dots \rangle$  represents an average over statistically-independent Monte Carlo measurements.

#### 2. Local Constraints

Figure 2 of the main text and Fig. S3 in this Supplemental Material clearly show characteristic “pinch-point” singularities in the equal-time structure factors for both dipole and quadrupole spin moments. These signatures provide direct evidence of an underlying Coulombic gauge structure within a given spin liquid manifold, which corresponds to a local divergence-free condition [11–13]. To capture the crossover from a high-temperature paramagnet to a low-temperature Coulombic spin liquid, we evaluate local constraints that explicitly measure the divergence-free condition [14].

The operator characterizing local constraints for spin-dipoles is defined as

$$\Gamma^S = \frac{1}{N} \sum_{\triangle} \left( \sum_i \|\mathbf{S}_i\|^2 - \frac{1}{4} \left\| \sum_i \mathbf{S}_i \right\|^2 \right), \tag{S23}$$

while for spin-quadrupoles, it is given by

$$\Gamma^Q = \frac{1}{N} \sum_{\triangle} \left( \sum_i \|\mathbf{Q}_i\|^2 - \frac{1}{4} \left\| \sum_i \mathbf{Q}_i \right\|^2 \right). \tag{S24}$$

The BBQ model not only supports Coulombic spin liquids with dominant fluctuations in either the dipolar or quadrupolar channels, but also allows for a spin liquid where dipoles and quadrupoles contribute equally. Due to the symmetry of the Hamiltonian, such fluctuations are particularly prominent near the antiferromagnetic  $SU(3)$  point at  $\phi = 0.25\pi$ . To evaluate the Coulomb law for these fluctuations, we define an operator characterizing the local constraint for the  $\mathcal{A}$  matrices, which, following Eq. (S8), is constructed by a linear combination of Eqs. (S23) and (S24):

$$\begin{aligned}
\Gamma^A &= \frac{1}{N} \sum_{\triangle} \left( \sum_i \left[ \|\mathbf{S}_i\|^2 + \|\mathbf{Q}_i\|^2 \right] - \right. \\
&\quad \left. \frac{1}{4} \left[ \left\| \sum_i \mathbf{S}_i \right\|^2 + \left\| \sum_i \mathbf{Q}_i \right\|^2 \right] \right).
\end{aligned} \tag{S25}$$

The associated susceptibilities of Eqs. (S23)–(S25) are given by

$$\chi[\Gamma^\rho] = \frac{N}{T} \left[ \langle (\Gamma^\rho)^2 \rangle - \langle \Gamma^\rho \rangle^2 \right] \tag{S26}$$

where  $\rho = \{S, Q, A\}$ . A summary of all relevant bond correlation functions and local constraints for each spin liquid are summarized in Tab. SI.

| spin liquid                             | spin moments | correlators and local constraints  | Eq.   |
|-----------------------------------------|--------------|------------------------------------|-------|
| nematic [ $\mathbb{RP}^2 \times U(1)$ ] | dipolar      | $\lambda_E^S$                      | (S21) |
| dipolar Coulombic [dC]                  | dipolar      | $\Gamma^S$                         | (S23) |
| dipolarcolorice [dCI]                   | dipolar      | $\lambda_{A_1}^S$                  | (S21) |
| $SU(3)$ coulombic [su3C]                | mixed        | $\Gamma^A$                         | (S25) |
| quadrupolar color ice [qCI]             | quadrupolar  | $\lambda_{A_1}^Q$                  | (S21) |
| quadrupolar Coulombic [qC]              | quadrupolar  | $\Gamma^Q$                         | (S24) |
| ferrimagnetic [Ferri $U(1)$ ]           | mixed        | $\lambda_{T_2}^S, \lambda_{T_2}^Q$ | (S21) |

Table SI. Summary of bond correlation functions and local constraints characterizing each spin liquid phase found in  $\mathcal{H}_{\text{BBQ}}$  of Eq. (S7). While all spin liquids exhibit crossovers from their high-temperature state, only the  $\mathbb{RP}^2 \times U(1)$  spin liquid undergoes a phase transition.

#### D. Variational energy minimization

To obtain the  $T = 0$  ground-state properties, we perform large-scale variational energy minimizations using the machine learning library JAX [2], accelerated by a NVIDIA® Jetson Orin Nano™ 8GB GPU compute module. We minimize the BBQ Hamiltonian,  $\mathcal{H}_{\text{BBQ}}$ , in Eq. (S7), by optimizing the variational parameters  $\theta_1, \theta_2, \phi_1, \phi_2$  and  $\phi_3$  in Eq. (S4) at each site on the pyrochlore lattice. This is achieved using the optimizer “Adam” within the gradient processing and optimization library “Optax” [15]. Simulations are initialized from relevant ordered and disordered states, as well as random configurations, for finite-size clusters with cubic symmetry and periodic boundary conditions. The optimization process for each set of model parameter involved about 10,000 optimization steps.

#### E. $U(3)$ Monte Carlo simulation

We perform semiclassical Monte Carlo simulations following the  $U(3)$  formalism (u3MC) introduced in [1] to evaluate the finite-temperature properties of  $\mathcal{H}_{\text{BBQ}}$  [Eq. (S7)]. The  $\mathcal{A}$  matrices, defined locally at each lattice site, are sampled using the Marsaglia construction [16] by randomly selecting parameters  $0 \leq \theta_1, \theta_2 \leq 1$  and  $0 \leq \phi_1, \phi_2 < 2\pi$ , as described in Eq. (S4). Following the standard single-spin flip Metropolis algorithm [17], new spin states are accepted or rejected after the evaluation of local bond energies.

In the actual simulations, a single u3MC step consists of  $N$  local spin-flip attempts (with  $N$  the total number of sites) at randomly chosen sites within a finite-size cluster of cubic symmetry and periodic boundary conditions. To reduce the autocorrelation time, we use the replica-exchange method (parallel tempering) [18–20], initiated every 100 MC steps. Thermodynamic quantities are averaged over  $1 \times 10^5$  statistically independent samples, after using  $5 \times 10^5$  steps for simulated annealing from high temperature and additional  $5 \times 10^5$  MC steps for thermalization.

#### F. Molecular dynamics simulation

To obtain dynamical structure factors for the spin-1 bilinear biquadratic model on the pyrochlore lattice we numerically integrate the equations of motion in Eqs. (S13) and (S19). We start by generating statistically independent and sufficiently thermalized  $\mathcal{A}$ -matrix configurations using u3MC simulations, as outlined in Sec. IE. For each  $\mathcal{A}$  matrix configuration, we generate a time series  $\{\mathcal{A}_{i\beta}^\alpha(t)\}$ , by numerically integrating the the equations of motion given in Eqs. (S13) and (S19) using a fourth-order Runge-Kutta method [21, 22]. The Fourier transform of this time series is then computed with

$$m_{\mathcal{A}}^{\alpha}_{\beta}(\mathbf{q}, \omega) = \frac{1}{\sqrt{N_t N}} \sum_i \sum_t^{N_t} e^{i\mathbf{q} \cdot \mathbf{r}_i} e^{i\omega t} \mathcal{A}_{i\beta}^\alpha(t), \quad (\text{S27})$$

using a Fast Fourier Transform (FFT) [23]. To minimize numerical artifacts such as the Gibbs phenomenon, and to mimic frequency resolution from experiment, we convolute numerical data with a Gaussian envelope [24].

Since  $m_{\mathcal{A}}^{\alpha}_{\beta}(\mathbf{q}, \omega)$  contains the information of all fluctuations allowed for a spin-1 moment, we separate the contributions from dipole and quadrupole moments via

$$m_S^{\alpha}(\mathbf{q}, \omega) = -i \sum_{\beta, \gamma} \epsilon_{\beta}^{\alpha \gamma} m_{\mathcal{A}}^{\beta}_{\gamma}(\mathbf{q}, \omega), \quad (\text{S28})$$

$$m_Q^{\alpha}_{\beta}(\mathbf{q}, \omega) = -m_{\mathcal{A}}^{\alpha}_{\beta}(\mathbf{q}, \omega) - m_{\mathcal{A}}^{\beta}_{\alpha}(\mathbf{q}, \omega) + \frac{2}{3} \delta_{\beta}^{\alpha} \sum_{\gamma} m_{\mathcal{A}}^{\gamma}_{\gamma}(\mathbf{q}, \omega). \quad (\text{S29})$$

Finally, the dynamical structure factors for dipole and quadrupole channels follows

$$S_{\rho}(\mathbf{q}, \omega) = \left\langle \sum_{\alpha\beta} |m_{\rho}^{\alpha}_{\beta}(\mathbf{q}, \omega)|^2 \right\rangle, \quad (\text{S30})$$

where  $\rho = \{S, Q, \mathcal{A}\}$ , and  $\langle \dots \rangle$  represents an average over statistically-independent time series.

In the actual simulations, we evolve replicas over approximately  $N_t = 6000$  time steps with a time increment of  $\delta t = 0.008 \text{ meV}^{-1}$ . For the Fourier transform in time, unless stated otherwise, we use every 20th time snapshot and apply a Gaussian envelope to the signal to reduce numerical artifacts, resulting in a frequency resolution with a full width at half maximum (FWHM) of 0.2 meV. Results were averaged over 500 – 1000 statistically independent time series for cluster sizes with a linear dimension of  $L = 8$  ( $N = 8192$ ).

## II. VARIATIONAL GROUND STATE PHASE DIAGRAM

To determine the ground-state phase diagram in Fig. 2 of the main text, we perform variational energy minimization of  $\mathcal{H}_{\text{BBQ}}$  in Eq. (S7), as discussed in Sec. ID. The coupling constants are parametrized with

$$(J, K) = (\cos \phi, \sin \phi). \quad (\text{S31})$$

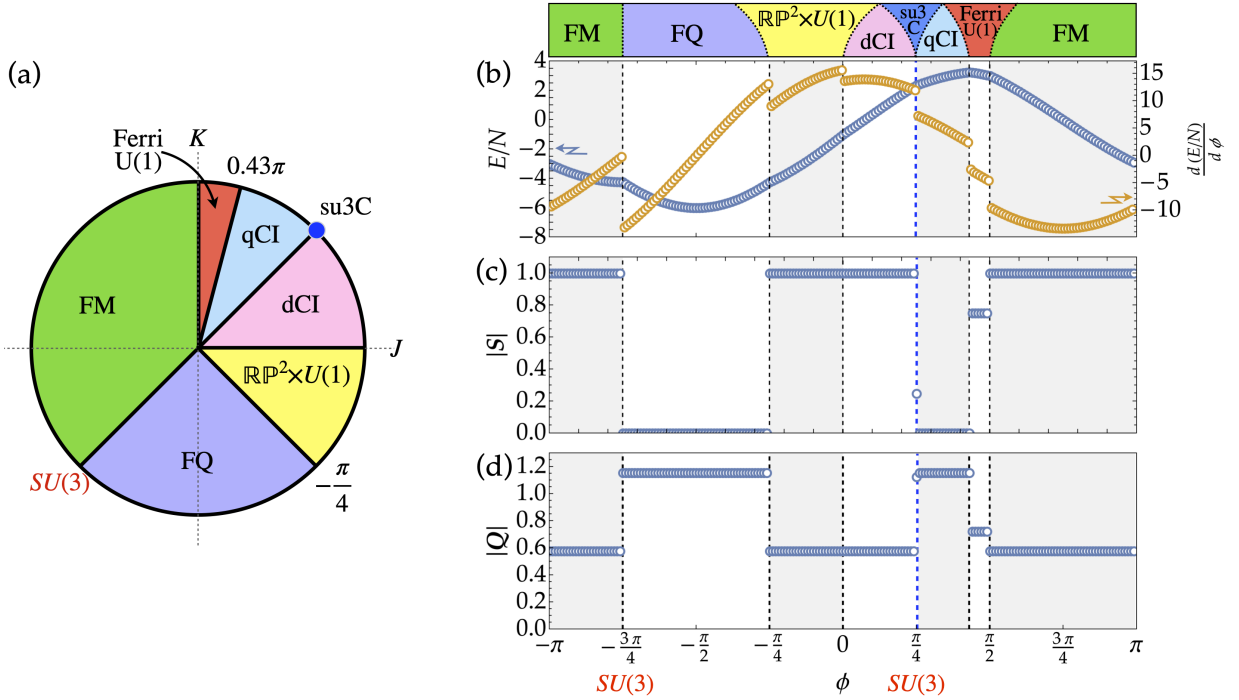

Figure S2. Ground states of the bilinear biquadratic (BBQ) model as function of model parameters, and character of associated spin moments. (a) Ground-state phase diagram of  $\mathcal{H}_{BBQ}$  [Eq. (S7)], as a function of the parameter  $\phi$  [Eq. (S31)]. (b) Energy per site,  $E/N$ , and its derivative,  $d(E/N)/d\phi$ . (c) Averaged spin-dipole norm,  $|S|$  [Eq. (S32)]. (d) Averaged spin-quadrupole norm,  $|Q|$  [Eq. (S33)]. Discontinuities in  $d(E/N)/d\phi$  indicate that all phases are separated by first-order phase transitions. Calculations were performed using variational energy minimization techniques (see Sec. ID) for finite-size clusters of linear dimension  $L = 20$  and total number of sites  $N = 128,000$ .

and finite-size clusters are simulated under periodic boundary conditions, preserving the cubic symmetry of the pyrochlore lattice. Simulations are carried out for clusters with a linear system size of  $L = 20$ , containing a total number of sites  $N = 16L^3 = 128,000$ .

In Fig. S2(a) we present the ground-state phase diagram as function of normalized model parameters  $J$  and  $K$ . The model stabilizes magnetically ordered, ferromagnetic (FM) and ferroquadrupolar (FQ) spin nematic phases over a wide range of model parameters. In the region where  $J$  and  $K$  frustrate the model, we observe in total five different spin liquid phases, namely the  $\mathbb{RP}^2 \times U(1)$  nematic spin liquid, dipolar color ice (dCI), the  $SU(3)$  Coulombic spin liquid (su3C) at the singular  $SU(3)$  point ( $\phi = 0.25\pi$ ), the quadrupolar color ice (qCI), and the ferrimagnetic (ferri)  $U(1)$  spin liquid. Phase boundaries are determined from the normalized energy,  $E/N$ , and its derivative,  $d(E/N)/d\phi$ , as shown in panel S2(b). Correspondingly, panels S2(c) and S2(d), display the average spin-dipole norm,  $|S|$ , and the average spin-quadrupole norm,  $|Q|$ , calculated as

$$|S| = \frac{1}{N} \sum_i |S_i|, \quad (S32)$$

$$|Q| = \frac{1}{N} \sum_i |Q_i|, \quad (S33)$$

with the definitions of spin-dipole and spin-quadrupole components provided in Eqs. (S10) and (S11).

Discontinuities in  $d(E/N)/d\phi$  confirm that all phases in this model are separated by first-order phase transitions. Each phase exhibits a constant value of the spin-dipole norm  $|S|$ , indicating that the spin length remains unchanged with each phase upon varying model parameters. Phases such as FM,  $\mathbb{RP}^2 \times U(1)$  and dCI are purely dipolar, whereas FQ, and qCI are purely quadrupolar. The Ferri  $U(1)$  phase exhibits  $|S| = 0.75$ , which arises because one spin moment per tetrahedron is quadrupolar, while the remaining three spins are dipolar.

### III. SPIN LIQUID PHASES AND THEIR PINCH-POINTS IN THE $(h, k, 0)$ PLANE

In this section, we supplement the energy-integrated structure factors shown in Fig. 3 of the main text for the  $(h, h, l)$  with results for the  $(h, k, 0)$  plane. Figure S3 shows the corresponding structure factors for the same model parameters as used in Fig. 3. In every spin liquid phase, characteristic pinch-point singularities appear in either the spin-dipole or spin-quadrupole channel, directly indicating the presence of an underlying divergence-free condition in the corresponding



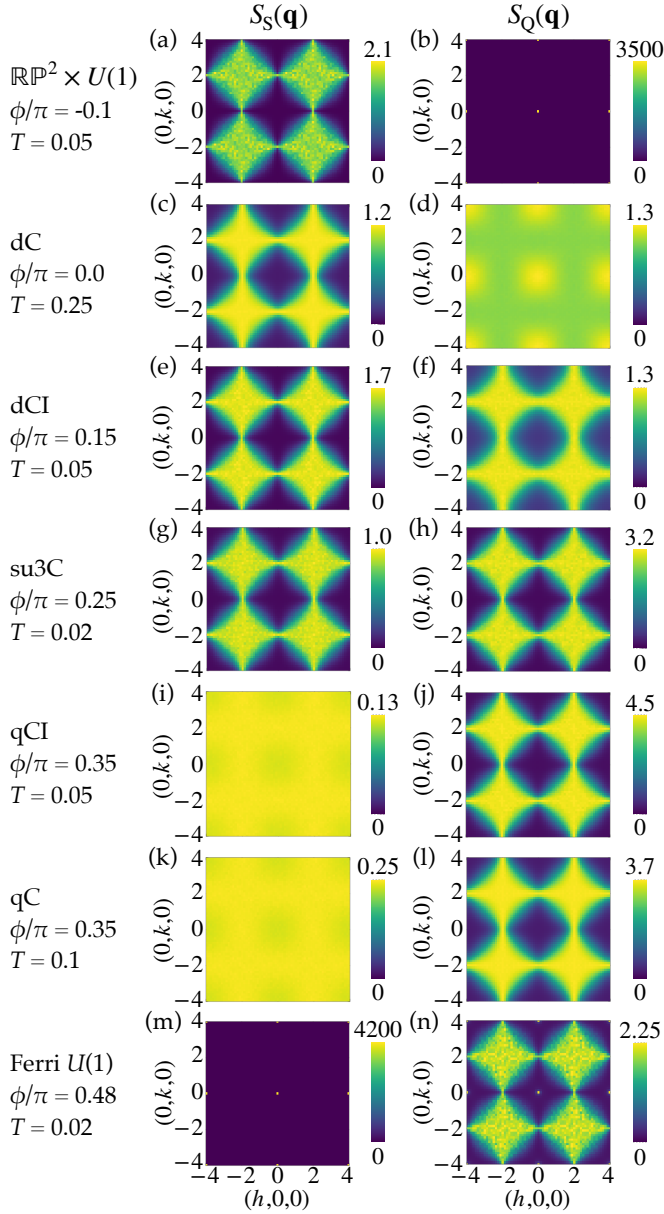

Figure S3. Equal-time structure factors within the  $(h, k, 0)$  plane for the seven spin liquid phases found in the spin-1 bilinear bi-quadratic model on the pyrochlore lattice (see Fig. 3 of the main text and Table S1). *Left column:* spin-dipoles,  $S_S(\mathbf{q})$ . *Right column:* spin-quadrupoles,  $S_Q(\mathbf{q})$ . All spin-liquids exhibit pinch-point singularities at Brillouin-zone centers, directly indicating the presence of local divergence-free conditions. Notably, the Coulombic liquid at the antiferromagnetic  $SU(3)$  point (su3C) is unique, displaying pinch-points in both channels. The dipolar color ice (dCI) and  $\mathbb{RP}^2 \times U(1)$  phases exhibit pinch-points in the spin-dipole channel, while the quadrupolar color ice (qCI) and ferrimagnetic Coulombic [Ferri  $U(1)$ ] phases show pinch-points in the spin-quadrupole channel. Results were obtained from  $U(3)$  Monte Carlo (u3MC) simulations, for cubic clusters with periodic boundary conditions and linear dimension  $L = 8$  ( $N = 8192$ ).

Coulomb gauge field, namely

$$\nabla \mathbf{m}_S = \sum_i \mathbf{S}_i = 0 \quad \forall \triangle, \quad (\text{S34})$$

$$\nabla \mathbf{m}_Q = \sum_i \mathbf{Q}_i = 0 \quad \forall \triangle. \quad (\text{S35})$$

for spin-dipoles and spin-quadrupoles, respectively.

A particularly interesting case is the su3C spin liquid, where the  $SU(3)$  symmetry of the Hamiltonian makes dipoles and quadrupoles equivalent. As a result, this spin liquid exhibits pinch points in both channels simultaneously. The distribution of pinch points in the dipole and quadrupole channels follows a somewhat symmetric pattern around this  $SU(3)$  point. Specifically, the dCI, dC, and  $\mathbb{RP}^2 \times U(1)$  phases display pinch points in the dipole channel, while the qCI, qC, and Ferri  $U(1)$  phases exhibit pinch points in the quadrupole channel. Interestingly, in the  $\mathbb{RP}^2 \times U(1)$  and Ferri  $U(1)$  phases, one channel features pinch points while the other shows Bragg peaks, providing valuable examples of (semi-) classical Coulombic spin liquids which coexist with a spontaneously broken symmetry.

#### IV. THERMODYNAMICS FOR $\mathbb{RP}^2 \times U(1)$ AND DIPOLAR COLOR ICE

$\text{NaCaNi}_2\text{F}_7$  is a spin-1 magnet in which magnetic dipole and quadrupole moments are unavoidable and appear to play a crucial role for its physical properties. The simplest and most general model incorporating interactions between these moments is the BBQ model, commonly expressed in Eq. (1) of the main text and formulated within the  $U(3)$  formalism in Eq. (S7) of this Supplemental Material. As discussed in Fig. 1 of the main text, finite quadrupolar interactions immediately drive the system into one of two distinct spin liquid phases: the  $\mathbb{RP}^2 \times U(1)$  nematic spin liquid for  $K < 0$  and the dipolar color ice for  $K > 0$ . In Figs. 4 and 5 of the main text, we compare the dynamical signatures of these two spin liquid phases and propose that the characteristically gapped spin structure factor observed in  $\text{NaCaNi}_2\text{F}_7$  may originate from nonzero negative biquadratic interactions ( $K < 0$ ).

As a supplement to the dynamical structure factors presented in Fig. 4 of the main text, we show the thermodynamic properties of the  $\mathbb{RP}^2 \times U(1)$  and dCI phases for the same model parameters. Figure S4 presents thermodynamic observables at  $\phi \approx -0.1\pi$ , with

$$J = 2.4 \text{ meV}, \quad K = -0.8 \text{ meV}, \quad (\text{S36})$$

which stabilizes the  $\mathbb{RP}^2 \times U(1)$  nematic spin liquid at low temperatures. The specific heat, shown in Fig. S4(a), exhibits a sharp first-order phase transition into the  $\mathbb{RP}^2 \times U(1)$  nematic spin liquid at  $T_c = 3.05(5)$  K. As shown in Fig. S4(b), this transition is accompanied by a diverging nematic order parameter,

$$m_Q = \sqrt{\sum_{\alpha\beta} \left( \sum_i Q_{i\beta}^\alpha \right)^2}, \quad (\text{S37})$$

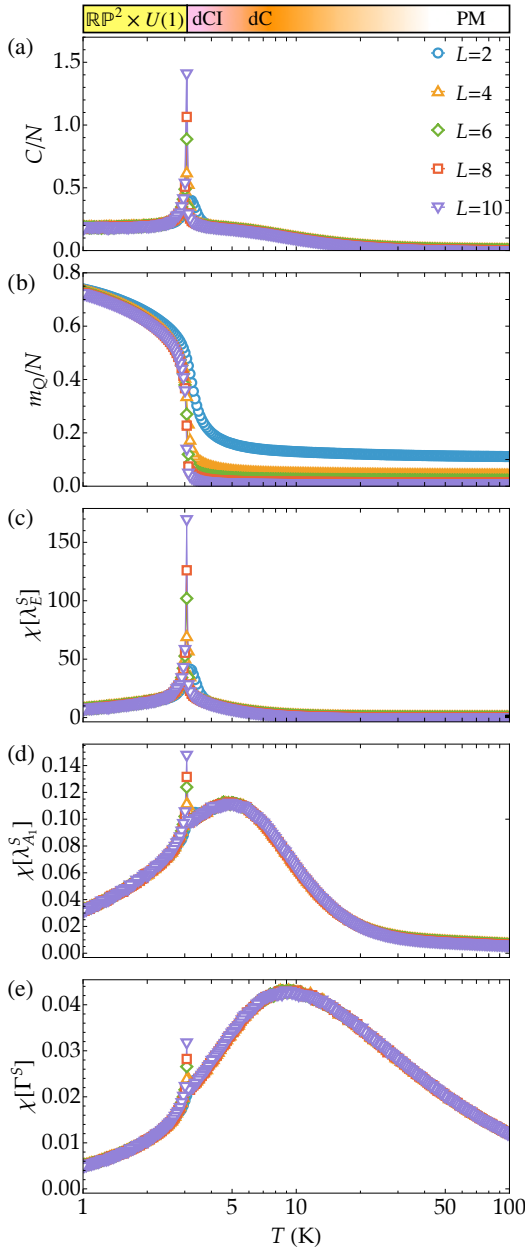

Figure S4. Thermodynamic observables for the BBQ model,  $\mathcal{H}_{\text{BBQ}}$  [Eq. (S7)], at model parameters in Eq. (S36) that stabilize the  $\mathbb{RP}^2 \times U(1)$  spin liquid at low temperatures. Shown are (a) specific heat, (b) nematic order parameter [see Eq. (S37)], (c) susceptibility of the dipolar bond-order parameter with irrep E, (d) susceptibility of the dipolar bond-order parameter with irrep  $A_1$  [see Eq. (S22)], and (e) susceptibility of the local constraints for spin-dipoles [see Eq. (S26)]. All observables exhibit a singular behaviour at the phase transition into the  $\mathbb{RP}^2 \times U(1)$  spin liquid at  $T_c = 3.05(5)$  K. Additionally, (d) and (e) reveal broad crossovers spanning multiple regimes, from the high-temperature paramagnet (PM) to the dipolar Coulombic (dC) spin liquid, and subsequently to dipolar color ice (dCI).

with  $Q_{i\beta}^\alpha$  defined in Eq. (S6).

The  $\mathbb{RP}^2 \times U(1)$  spin liquid is symmetric under the bond

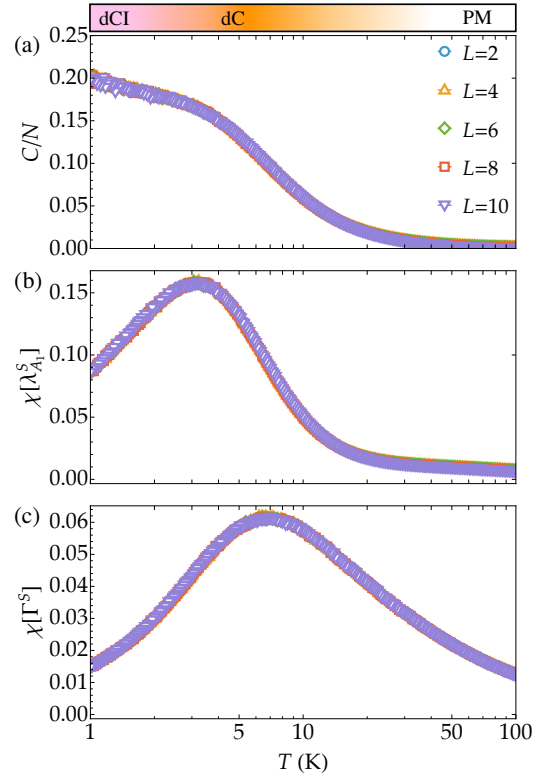

Figure S5. Thermodynamic observables for the BBQ model,  $\mathcal{H}_{\text{BBQ}}$  [Eq. (S7)], at model parameters in Eq. (S38) that stabilize the dipolar color ice (dCI) spin liquid at low temperatures. Shown are (a) specific heat, (b) the susceptibility of the dipolar bond-order parameter with irrep  $A_1$  [see Eq. (S22)], and (c) the susceptibility of the local constraints for spin-dipoles [see Eq. (S26)]. Observables show no signatures of a phase transition, only crossovers from the high-temperature paramagnet (PM) to dipolar Coulombic (dC) spin liquid, and subsequently to dipolar color ice (dCI).

irrep E [9]. Accordingly, we present the susceptibility of the bond correlation function,  $\chi[\lambda_E^S]$  [see Eq. (S22)], in Fig. S4(c), which exhibits a sharp singularity at the phase-transition temperature  $T_c$ . A weaker signature of this transition is also observed in the susceptibilities of the bond correlation function with irrep  $A_1$ ,  $\chi[\lambda_{A_1}^S]$ , and the local constraints for spin-dipoles,  $\chi[\Gamma^S]$  [see Eq. (S26)], as shown in Figs. S4(d) and S4(e), respectively. However, these correlators primarily capture system-size-independent crossovers over a broad temperature range, with peak maxima at approximately  $T_1 \approx 9$  K, and  $T_2 \approx 5$  K. This suggests a three-step evolution: an initial crossover from the high-temperature paramagnetic (PM) state into the dC spin liquid, followed by a second crossover into the dCI phase, and finally a first-order phase transition into the  $\mathbb{RP}^2 \times U(1)$  spin liquid.

In Fig. S5, we present thermodynamic observables for positive biquadratic exchange at  $\phi \approx 0.1\pi$ , with

$$J = 2.4 \text{ meV}, \quad K = 0.8 \text{ meV}, \quad (\text{S38})$$

which stabilize the dCI spin liquid at low temperatures. The specific heat in Fig. S5(a) shows no indication of a phase tran-

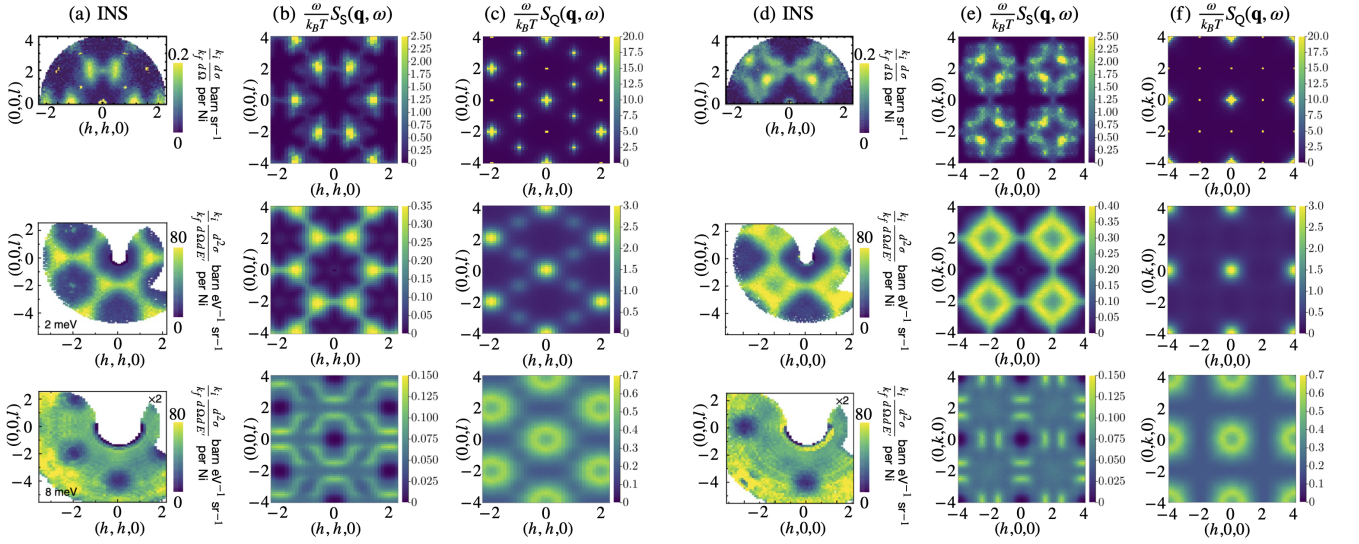

Figure S6. Qualitative comparison of dynamical structure factors with in the  $(h, h, l)$  (left) and  $(h, k, 0)$  (right) planes between experiment and theory. (a), (d) Inelastic neutron scattering (INS) data of  $\text{NaCaNi}_2\text{F}_7$  (taken from Ref. [25]). (b), (e) Dipolar structure factor from u3MD simulations for model parameters in Eq. (S39) at  $T \approx 1.8$  K. (c), (f) Corresponding quadrupolar structure factor from u3MD simulations. Simulations were averaged over  $l \pm 0.25$  and  $\omega \pm 0.2$  meV to mimic experimental conditions.

sition. Meanwhile, the susceptibilities of the dipolar bond correlation function,  $\chi[\lambda_{A_1}^S]$ , and the local constraints for spin-dipoles,  $\chi[\Gamma^S]$ , exhibit distinct crossovers over a broad temperature range. This suggests a gradual evolution from the high-temperature PM into the dC and eventually the dCI spin liquid phases as the temperature decreases. It is important to note that the dipolar color ice state has been associated with the development of octupolar correlations in the  $O(3)$  version of this model [26]. While our model differs slightly, a similar tendency may arise at low temperatures. A detailed investigation of octupolar correlations in this setting is left for future work.

The temperature evolution described in Figs. S4 and Figs. S5 is reflected in the finite-temperature phase diagram shown in Fig. 1 of the main text. Notably, this phase diagram is presented on a different temperature scale, consistent with the normalized model parameters in Eq. (S31).

## V. DYNAMICS OF $\text{NaCaNi}_2\text{F}_7$

In Fig. 5 of the main text, we compare the dynamical structure factor for the  $\mathbb{RP}^2 \times U(1)$  spin liquid phase with inelastic neutron scattering (INS) results for  $\text{NaCaNi}_2\text{F}_7$ . Simulations are performed for the BBQ model with anisotropic interactions,  $\mathcal{H}_{\text{NaCaNi}_2\text{F}_7}$  [see Eq. (S14)], using the following model

parameters

$$\begin{aligned}
 J_1 &= 2.4 \text{ meV}, \\
 J_2 &= 2.4 \text{ meV}, \\
 J_3 &= 0.15 \text{ meV}, \\
 J_4 &= -0.23 \text{ meV}, \\
 J_{2\text{nd}} &= -0.06 \text{ meV}, \\
 K &= -0.8 \text{ meV},
 \end{aligned} \tag{S39}$$

at  $T \approx 1.8$  K. Dynamical properties are obtained by integrating the equations of motion in Eq. (S19).

In Fig. S6, we complement the  $S(\mathbf{q}, \omega)$  signal shown in the main text by presenting energy line cuts within the  $(h, h, l)$  (left panel) and  $(h, k, 0)$  (right panel) planes. We fit the model parameters to qualitatively reproduce the dominant features observed in the INS data from Ref. [25] [shown in Figs S6(a) and S6(d)] with the corresponding features seen in the spin-dipole channel of our u3MD simulations [shown in Figs. S6(b) and S6(e)]. The signatures from quadrupolar excitations, which predominantly represent the gapless Goldstone mode excitations, are shown in Figs. S6(c) and S6(f).

We emphasize that our model is underconstrained in the sense that we consider only anisotropic interactions between dipoles while adjusting parameters to capture general trends in the presence of biquadratic exchange  $K$ . Future developments, such as self-consistent Gaussian approximations within the  $U(3)$  formalism [28], may allow for a more systematic treatment of all allowed anisotropies (including those between quadrupolar terms) to improve the quantitative agreement between simulation and experiment.

In Fig. S7, we present line cuts in frequency and momentum space from the simulation data shown in Fig. S6 and compare them to the INS data from Ref. [25, 27]. As shown in



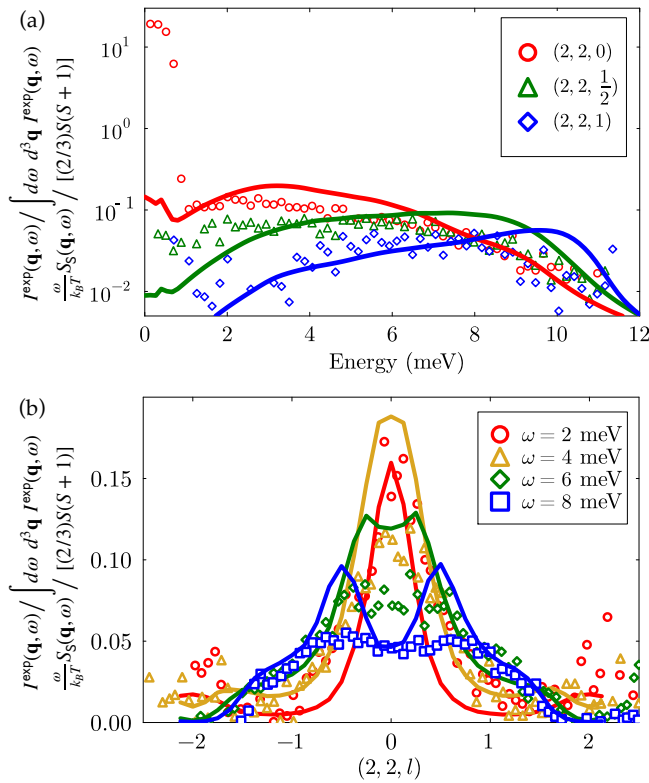

Figure S7. Comparison of dynamical dipole structure factor between experiment for NaCaNi<sub>2</sub>F<sub>7</sub> (taken from Ref. [27]), and u3MD simulations. (a) Frequency dependence on a log scale at fixed momentum  $\mathbf{q} = (2, 2, 0)$ ,  $(2, 2, \frac{1}{2})$  and  $(2, 2, 1)$ . (b) Momentum dependency at fixed frequency. Experimental data are shown as open markers, while u3MD simulations results are shown as solid lines.

Fig.S7(a), the simulation results qualitatively reproduce the experimental trends. Particularly, simulation results along the  $(2,2,0)$  path qualitatively reproduce the gapped nature of excitations observed in experiment — a feature that was not captured in previous  $O(3)$  simulations without biquadratic interactions [27]. Furthermore, the line cuts in Fig. S7(b) capture the main experimental features across all frequencies, reinforcing the validity of our approach.

- 
- [1] K. Remund, R. Pohle, Y. Akagi, J. Romhányi, and N. Shannon, Semi-classical simulation of spin-1 magnets, *Phys. Rev. Research* **4**, 033106 (2022).
  - [2] J. Bradbury, R. Frostig, P. Hawkins, M. J. Johnson, C. Leary, D. Maclaurin, G. Necula, A. Paszke, J. VanderPlas, S. Wanderman-Milne, and Q. Zhang, *JAX: composable transformations of Python+NumPy programs* (2018).
  - [3] A. Läuchli, F. Mila, and K. Penc, Quadrupolar Phases of the  $S = 1$  Bilinear-Biquadratic Heisenberg Model on the Triangular Lattice, *Phys. Rev. Lett.* **97**, 087205 (2006).
  - [4] H. Tsunetsugu and M. Arikawa, Spin Nematic Phase in  $S=1$  Triangular Antiferromagnets, *Journal of the Physical Society of Japan* **75**, 083701 (2006).
  - [5] H. Zhang and C. D. Batista, Classical spin dynamics based on  $SU(n)$  coherent states, *Phys. Rev. B* **104**, 104409 (2021).
  - [6] H. Yan, O. Benton, L. Jaubert, and N. Shannon, Theory of multiple-phase competition in pyrochlore magnets with anisotropic exchange with application to Yb<sub>2</sub>Ti<sub>2</sub>O<sub>7</sub>, Er<sub>2</sub>Ti<sub>2</sub>O<sub>7</sub>, and Er<sub>2</sub>Sn<sub>2</sub>O<sub>7</sub>, *Phys. Rev. B* **95**, 094422 (2017).
  - [7] K. Penc, N. Shannon, and H. Shiba, Half-magnetization plateau stabilized by structural distortion in the antiferromagnetic heisenberg model on a pyrochlore lattice, *Phys. Rev. Lett.* **93**, 197203 (2004).
  - [8] K. Penc, N. Shannon, Y. Motome, and H. Shiba, Symmetry considerations on the magnetization process of the heisenberg model on the pyrochlore lattice, *Journal of Physics: Condensed Matter* **19**, 145267 (2007).
  - [9] N. Shannon, K. Penc, and Y. Motome, Nematic, vector-multipole, and plateau-liquid states in the classical  $O(3)$  pyrochlore antiferromagnet with biquadratic interactions in applied magnetic field, *Phys. Rev. B* **81**, 184409 (2010).
  - [10] H. Yan, O. Benton, L. D. C. Jaubert, and N. Shannon, Rank-2  $U(1)$  Spin Liquid on the Breathing Pyrochlore Lattice, *Phys. Rev. Lett.* **124**, 127203 (2020).
  - [11] R. Moessner and J. T. Chalker, Low-temperature properties of classical geometrically frustrated antiferromagnets, *Phys. Rev. B* **58**, 12049 (1998).
  - [12] R. Moessner and J. T. Chalker, Properties of a Classical Spin Liquid: The Heisenberg Pyrochlore Antiferromagnet, *Phys. Rev. Lett.* **80**, 2929 (1998).
  - [13] C. L. Henley, Power-law spin correlations in pyrochlore antiferromagnets, *Phys. Rev. B* **71**, 014424 (2005).
  - [14] J. Greitemann, K. Liu, L. D. C. Jaubert, H. Yan, N. Shannon, and L. Pollet, Identification of emergent constraints and hidden order in frustrated magnets using tensorial kernel methods of machine learning, *Physical Review B* **100**, 174408 (2019).
  - [15] I. Babuschkin, K. Baumli, A. Bell, S. Bhupatiraju, J. Bruce,

- P. Buchlovsky, D. Budden, T. Cai, A. Clark, I. Danihelka, C. Fantacci, J. Godwin, C. Jones, R. Hemsley, T. Hennigan, M. Hessel, S. Hou, S. Kapturowski, T. Keck, I. Kemaev, M. King, M. Kunesch, L. Martens, H. Merzic, V. Mikulik, T. Norman, J. Quan, G. Papamakarios, R. Ring, F. Ruiz, A. Sanchez, R. Schneider, E. Sezener, S. Spencer, S. Srinivasan, L. Wang, W. Stokowiec, and F. Viola, *The DeepMind JAX Ecosystem* (2020).
- [16] G. Marsaglia, Choosing a Point from the Surface of a Sphere, *The Annals of Mathematical Statistics* **43**, 645 (1972).
- [17] N. Metropolis, A. W. Rosenbluth, M. N. Rosenbluth, A. H. Teller, and E. Teller, Equation of state calculations by fast computing machines, *The Journal of Chemical Physics* **21**, 1087 (1953).
- [18] R. H. Swendsen and J.-S. Wang, Replica Monte Carlo Simulation of Spin-Glasses, *Phys. Rev. Lett.* **57**, 2607 (1986).
- [19] K. Hukushima and K. Nemoto, Exchange Monte Carlo Method and Application to Spin Glass Simulations, *Journal of the Physical Society of Japan* **65**, 1604 (1996).
- [20] D. J. Earl and M. W. Deem, Parallel tempering: Theory, applications, and new perspectives, *Phys. Chem. Chem. Phys.* **7**, 3910 (2005).
- [21] E. Hairer, G. Wanner, and S. P. Nørsett, *Solving Ordinary Differential Equations I – Nonstiff Problems* (Springer Berlin Heidelberg, 1993).
- [22] W. H. Press, S. A. Teukolsky, W. T. Vetterling, and B. P. Flannery, *Numerical Recipes 3rd Edition: The Art of Scientific Computing*, 3rd ed. (Cambridge University Press, New York, NY, USA, 2007).
- [23] M. Frigo and S. G. Johnson, The Design and Implementation of FFTW3, *Proceedings of the IEEE* **93**, 216 (2005), special issue on “Program Generation, Optimization, and Platform Adaptation”.
- [24] G. B. Arfken and H. J. Weber, *Mathematical Methods for Physicists – International Edition*, 4th ed. (Academic Press, INC, 1995).
- [25] K. W. Plumb, H. J. Changlani, A. Scheie, S. Zhang, J. W. Krizan, J. A. Rodriguez-Rivera, Y. Qiu, B. Winn, R. J. Cava, and C. L. Broholm, Continuum of quantum fluctuations in a three-dimensional  $S = 1$  Heisenberg magnet, *Nature Physics* **15**, 54 (2019).
- [26] C. Cerkaskas, *Octupolar Ordering in the  $b > 0$  Bilinear-Biquadratic Heisenberg Model*, Master’s thesis, University of Waterloo (2019).
- [27] S. Zhang, H. J. Changlani, K. W. Plumb, O. Tchernyshyov, and R. Moessner, Dynamical Structure Factor of the Three-Dimensional Quantum Spin Liquid Candidate  $\text{NaCaNi}_2\text{F}_7$ , *Phys. Rev. Lett.* **122**, 167203 (2019).
- [28] K. Remund, O. Benton, and N. Shannon, unpublished.
